# Supplementary material for: Is your function low-dimensional?
Source: arXiv:1806.10057 source file (2018-11-02)
Supplement: Supplementary file 1 [file appendix.tex]

\section{Small net for noise attenuated linear juntas}~\label{sec:noise-attenuated}
In this section, we are going to prove the following theorem which essentially shows the existence of a small cover for noise stable linear juntas. To state this theorem, we will require one crucial fact about noise attenuated functions (due to Bakry and Ledoux~\cite{Bakry:94}) 
\begin{lemma}~\label{prop:gradient-bound}~
Let $f: \mathbb{R}^n \rightarrow [-1,1]$. Then, $P_t f$ is $C$-Lipschitz for $C = O(t^{-1/2})$. 
\end{lemma}

\begin{theorem}~\label{thm:net}
For any error parameter $\delta>0$, noise parameter $t>0$ and $k \in \mathbb{N}$, there is a set of functions $\mathsf{Cover}(t,k,\delta)$ (mapping $\mathbb{R}^k$ to $[-1,1]$) such that the following holds: 
\begin{enumerate}
\item Let $f: \mathbb{R}^n \rightarrow [-1,1]$ and $W$ be a $k$-dimensional space such that $P_t$ is $O(\epsilon)$-close to a $W$-junta. Further, $(w_1, \ldots, w_k)$ be any orthonormal basis of $W$. Then, $P_t f$ is $O(\delta)$-close to $h(\langle w_1, x \rangle, \ldots, \langle w_k, x \rangle)$ for some $h \in \mathsf{Cover}(t,k,\epsilon)$. 
\item The size of the set $\mathsf{Cover}(t,k,\epsilon)$ is bounded by 
$O\big( \frac{k \cdot \log(1/\delta)}{\sqrt{t} \cdot \delta}\big)^k$. 
\item Every function $ h \in mathsf{Cover}(t,k,\delta)$ is \emph{approximately Lipschitz} in the following sense:  
\[
\Vert_2 h(x) - h(y) \Vert_2 \le \Vert x - y \Vert_2 \cdot 
\]
\end{enumerate}
\end{theorem}

\section{Small net for juntas with bounded surface area}

\begin{proposition}~\label{prop:sing-value}
Let $A \in\mathbb{R}^{\ell \times \ell}$ matrix such that for any $1 \le j\le \ell$, $\dist(a_j, A_{j-1})) \ge \delta$ where $a_j$ is the $j^{th}$ column of $A$ and $A_j$ is the column span of the first $j$ columns. Then, for {\color{red}{$\eta = \delta^{-k}$}}\anote{this probably needs to change}, given the inner products of $\langle a_i, a_j \langle$ for all $(i,j)$ up to additive error $\eta$, 
the algorithm \textsf{Robust-linear-independence} has the following guarantee: 
\begin{itemize}
\item If the matrix $A$ satisfies the above conditions, 
then the algorithm outputs \textsf{yes}. 
\item If the algorithm outputs \textsf{yes}, then $\mathsf{dist}(a_j, A_{j-1}) \ge \delta/2$. 
\end{itemize} 
\end{proposition}
\begin{proof}
{\color{red}This proposition is supposed to basically say that with good enough accuracy, we can check whether the vectors we have gotten are $\eta$-linearly independent}
\end{proof}

\subsection{Small-covers for Lipschitz functions}
\begin{lemma}~\label{lem:Lipschitz-cover}
For any error parameter $\epsilon>0$, surface area $s$ and $k \in \mathbb{N}$, there is a net $\mathsf{Net}_{s,k,\epsilon}$ consisting of functions mapping $\mathbb{R}^k \rightarrow [-1,1]$ such that the following holds: Let $g: \mathbb{R}^n \rightarrow [-1,1]$ and let $P_{t_1} g$ be $\epsilon$-close to a $W$-junta where $\mathsf{dim}(W)=k$. 
Let $v_1, \ldots, v_k$ be an orthonormal basis of $W$. Then, there exists $h \in \mathsf{Net}_{s,k,\epsilon}$ such that $P_{t_1} g$ is $O(\epsilon)$-close to $h(\langle v_1, x\rangle, \ldots, \langle v_k ,x \rangle)$. 
\end{lemma}

\begin{proof}

\end{proof}

\begin{lemma}~\label{lem:net-1}
For any $C, \delta>0$ and $k \in \mathbb{N}$, there is a set $\mathsf{Net}_{k,C,\delta}$  consisting of functions mapping $\mathbb{R}^k \mapsto [-1,1]$ of size  $O\big(\frac{k \cdot C \cdot \log(1/\delta)}{\delta}\big)^k$ 
such that for any function $g: \mathbb{R}^k \rightarrow [-1,1]$ which is $C$-Lipschitz, there is a function $h \in \mathsf{Net}_{k,C,\delta}$, $\mathbf{E}[|g(x) - h(x)|] =\delta/9$. 
\end{lemma}
\begin{proof}
Let $\mathcal{B}  = \{x: \Vert x \Vert_2 \le \sqrt{k} \cdot \log (100/\delta)\}$. Now, let $\mathcal{A} \subseteq \mathcal{B}$ be defined as the set of points each of whose coordinates is an integral multiple of $\eta=\frac{\delta}{10 \cdot C \cdot \sqrt{k}}$. For $f: \mathbb{R}^n \rightarrow [-1,1]$, we now define $f_{\mathsf{int}}$ as follows: 
\begin{enumerate}
\item For any point $x \not \in \mathcal{B}$, $f_{\mathsf{int}}(x)=0$. 
\item For any point $x \in \mathcal{A}$, $f_{\mathsf{int}}(x)$ is defined to be the closest integral multiple of $\delta/100$ to $f(x)$. 
\item For any point $x \in \mathcal{B} \setminus \mathcal{A}$, $f_{\mathsf{int}}(x) = f(y)$ where $y$ is the point in $\mathcal{A}$ closest to $x$. 
\end{enumerate}
We next observe that for any $x \in \mathcal{B}$, if $y$ denotes the closest point in $\mathcal{A}$, then 
\[
|f(x) - f_{\mathsf{int}}(x)| \le |f(x) - f(y)| + |f(y) - f_{\mathsf{int}}(y)| \le \frac{\delta}{100} + \frac{\delta}{10} \le \frac{11 \delta}{100}. 
\]
The above uses the fact that $f$ is $C$-Lipschitz and the $\ell_2$ distance between $x$ and $y$ is bounded by $\frac{\delta}{10C}$. Now, observe any function of the form $f_{\mathsf{int}}$ can be specified by its value on the set $\mathcal{A}$ and further these values are one of $O(1/\delta)$ possiblities. Thus, if we define $ \mathsf{Net}_{k,C,\delta}$ as the set of all such functions, we obtain the lemma. Since $|\mathcal{A}| =O\big(\frac{k \cdot C \cdot \log(1/\delta)}{\delta}\big)^k$, we obtain the bound on the size of $ \mathsf{Net}_{k,C,\delta}$.
\end{proof}

\begin{lemma}~\label{lem:Lip-1}
Let $f: \mathbb{R}^n \rightarrow [-1,1]$ be a $c$-Lipschitz function. Further, let $g: \mathbb{R}^n \rightarrow [-1,1]$ be a $W$-junta such that $f$ is $O(\epsilon)$-close to $g$. Then, there is a function $f_W:\mathbb{R}^n \rightarrow [-1,1]$ which is $c$-Lipschitz and $W$-junta which is $O(\epsilon)$-close to $f$. 
\end{lemma}
\begin{proof}
Reorient the axes so that $W$ is the space spanned by the first $\ell$-axes. Let us define the $W$-junta $f_{W}: \mathbb{R}^n \rightarrow [-1,1]$ defined as 
\[
f_W(x) = \mathbf{E}_{y_{\ell+1}, \ldots, y_n} [f(x_1, \ldots, x_\ell, y_{\ell+1}, \ldots, y_n)
\]
For any fixed choice of $x_1, \ldots, x_\ell$, we have
\[
\mathbf{E}_{x_{\ell+1}, \ldots, x_n}[|f(x) - f_W(x)|] \leq \mathbf{E}_{x_{\ell+1}, \ldots, x_n}[|f(x) - g(x)|]  +|g(x) - f_W(x)|. 
\]
However, the second term can be bounded as 
\[
|g(x) - f_W(x)| = \big| g(x) - \mathbf{E}{x_{\ell+1}, \ldots, x_n}[f(x_1, \ldots,x_\ell, x_{\ell+1} , \ldots, x_n)] \big|  \le \mathbf{E}{x_{\ell+1}, \ldots, x_n} \big[ \big| g(x) - f(x) \big|\big]
\]
The last inequality is simply Jensen's inequality. Combining these two, we get 
\begin{equation}~\label{eq:junta-diff}
\mathbf{E}_{x_{\ell+1}, \ldots, x_n}[|f(x) - f_W(x)|] \leq2 \cdot \mathbf{E}_{x_{\ell+1}, \ldots, x_n}[|f(x) - g(x)|]. 
\end{equation}
This in turn implies that 
\begin{equation}~\label{eq:junta-diff-1}
\mathbf{E}_{x_{1}, \ldots, x_n}[|f(x) - f_W(x)|] \leq2 \cdot \mathbf{E}_{x_{1}, \ldots, x_n}[|f(x) - g(x)|] \leq 2\cdot \epsilon. 
\end{equation}
Finally, we see that 
\begin{eqnarray*}
|f_W(x) - f_W(y)|  &=& \big| \mathbf{E}_{x_{\ell+1}, \ldots, x_n}[f(x_1, \ldots, x_\ell, x_{\ell+1} , \ldots, x_n) - f(y_1, \ldots, y_\ell, x_{\ell+1},\ldots, x_n)] \\
&\leq&  \mathbf{E}_{x_{\ell+1}, \ldots, x_n} \big[ \big| f(x_1, \ldots, x_\ell, x_{\ell+1} , \ldots, x_n) - f(y_1, \ldots, y_\ell, x_{\ell+1},\ldots, x_n) \big| \big] \\
&\le&  \mathbf{E}_{x_{\ell+1}, \ldots, x_n} [ C \cdot \Vert  (x_1, \ldots, x_\ell) - (y_1, \ldots, y_\ell) \Vert_2] \le C \Vert x -y\Vert_2. 
\end{eqnarray*}
This finishes the proof. 
\end{proof}

\begin{proof}
First, we apply Proposition~\ref{prop:gradient-bound} to observe that $P_t f$ is $\kappa=O(t^{-1/2})$-Lipschitz. Since $P_t f$ is $O(\epsilon)$-close to a $W$-junta, we obtain that $P_t f$ is $O(\epsilon)$ close to a $W$-junta $g$ which is $\kappa$-Lipschitz (follows from Lemma~\ref{lem:Lip-1}). Let $ \mathsf{Cover}(t,k,\epsilon)=\mathsf{Net}_{k,\kappa,\epsilon}$ (where $\mathsf{Net}_{k,\kappa,\epsilon}$ in the set from Lemma~\ref{lem:Lipschitz-cover}). By a rotation of the coordinates, it follows from the definition of $ \mathsf{Cover}(t,k,\epsilon)$ that there exists $h \in\mathsf{Cover}(t,k,\epsilon)$ such that $h( \langle w_1, x \rangle, \ldots, \langle w_k, x \rangle)$ is $O(\epsilon)$ close to $P_tf$. This finishes the proof. The upper bound on the size of the set $\mathsf{Cover}(t,k,\epsilon)$ follows from Lemma~\ref{lem:Lipschitz-cover}. 
\end{proof}
\begin{lemma}~\label{lem:apx-ortho}
For $f: \mathbb{R}^n \rightarrow [-1,1]$ and $t>0$, let $(y_1, \ldots, y_\ell)$ be $\gamma$-linearly independent for $h = P_t f$. Let $v_i = D_{y_i} h(y_i)$ and let $V = \mathsf{span}(v_1, \ldots, v_\ell)$. 
For any error parameter $\tau>0$ and for $T  = T(\tau, t, \gamma)$ defined as 
\[
T(\tau, t, \gamma) =  \mathsf{poly} \bigg( \frac{1}{t}, 2 \frac{k}{\tau \cdot \sqrt{t}} \cdot \big( \frac{k}{2\cdot \gamma \cdot \sqrt{t}}\big)^{3k+3}\bigg)
\]
we can make $T$ queries to oracle for $f$ and obtain numbers 
 $\{\alpha_{i,j}\}_{1\le i,j \le \ell}$ such that the following holds:
\begin{enumerate}
\item For $\xi ( t, \gamma)$ defined as 
\[
\xi ( t, \gamma) = \bigg(\frac{2 k }{\gamma \cdot \sqrt{t}}\bigg)^{\frac{k+1}{2}} \cdot k^{3/2} \cdot \frac{1}{\sqrt{t}}, 
\]
 we have 
$|\alpha_{i,j}| \le \xi ( t, \gamma)$. 
\item There is an orthonormal basis $(w_1, \ldots, w_\ell)$ of $(Dh_{y_1}(y_1), \ldots, Dh_{y_\ell}(y_\ell))$ such that for $$\Vert w_{i} - \sum_{j}\alpha_{i,j} Dh_{y_j}(y_j) \Vert_2 \le \tau.$$ 
\end{enumerate}
\end{lemma}
\begin{proof}
We first invoke Lemma~\ref{lem:inner-product-1} to obtain that with $T$ queries, we can compute numbers $\beta_{i,j}$ with the following guarantee: 
\[
\big| \beta_{i,j} - \langle D_{y_i} h(y_i) , D_{y_j} h(y_j) \rangle \big| \le  2 \frac{\tau \cdot \sqrt{t}}{k } \cdot \bigg( \frac{\gamma \cdot \sqrt{t}}{2\cdot k }\bigg)^{3k+3}
\]
Now, observe that because $(y_1, \ldots, y_\ell)$ are $\gamma$-linearly independent, hence as vectors 
$(Dh_{y_1}(y_1), \ldots, Dh_{y_\ell}(y_\ell))$ are 
$(t^{-1/2}, \gamma)$ linearly independent. We can now apply Proposition~\ref{prop:linear} to obtain the numbers the numbers $\{\alpha_{i,j}\}$ promised here. 
\end{proof}

\begin{proposition}~\label{prop:linear}
Let $v_1, \ldots, v_\ell$ be a $(\eta, \gamma)$-linearly independent vectors. Then, for $\epsilon>0$, $\lambda(\epsilon,\eta, \gamma)$ defined as 
$$
\lambda= 2 \frac{\epsilon}{\ell \cdot \eta} \cdot \big( \frac{\gamma}{2\cdot \ell \cdot \eta}\big)^{3\ell+3}, 
$$ given numbers $\{\beta_{i,j}\}_{1\le i,j \le \ell}$ such that $|\beta_{i,j} - \langle v_i, v_j \rangle| \le \lambda$, we can compute numbers $\{\alpha_{i,j}\}_{1\le i,j \le \ell}$ such that: 
\begin{enumerate}
\item For $\xi ( \eta, \gamma)$ defined as 
\[
\xi ( \eta, \gamma) = \bigg(\frac{2 \ell \eta}{\gamma}\bigg)^{\frac{\ell+1}{2}} \cdot \ell^{3/2} \cdot \eta, 
\]
 we have 
$|\alpha_{i,j}| \le \xi ( \eta, \gamma)$.
\item There is an orthonormal basis $(w_1, \ldots, w_\ell)$ of $\mathsf{span}(v_1, \ldots, v_\ell)$ such that for $\Vert w_{i} - \sum_{j}\alpha_{i,j} v_j \Vert_2 \le \epsilon$. 
\end{enumerate}
\end{proposition}
\begin{proof}
 Consider the symmetric matrix $\Sigma\in\mathbb{R}^{\ell \times \ell}$ defined as $\Sigma_{i,j} = \langle v_i, v_j \rangle$. By Proposition~\ref{prop:sing-1}, $\Sigma$ is non-singular. Define the matrix $\Gamma = \Sigma^{-1/2}$. It is easy to see that the columns of 
 $V \cdot \Sigma^{-1/2}$ form an orthonormal basis of $\mathsf{span}(v_1, \ldots, v_\ell)$. Here $V = [v_1 | \ldots  | v_\ell]$. Of course, we cannot compute the matrix $\Sigma$ exactly and consequently, we cannot compute the matrix $\Sigma^{-1/2}$ either.

 Instead, we can compute a 
 $\widetilde{\Sigma}$ (which is also symmetric) 
 such that $\Vert \widetilde{\Sigma} - \Sigma \Vert_F\le \ell \cdot \lambda$.  Now, for an error parameter $\delta$ to be fixed, assume that
 $$
 \ell \cdot \lambda \le \delta  \cdot \sigma_{\min}(\Sigma)  = \delta \cdot \sigma_{\min}^2(V) \le \delta \cdot \bigg(\frac{ \gamma}{2 \cdot \ell \cdot \eta}\bigg)^{2\ell+2}.
 $$
 Here the second inequality, uses Proposition~\ref{prop:sing-1}. Now, we apply the matrix perturbation bound (Corollary~\ref{corr:mat-perturb}) 
 (i.e., here we set $c = \big( \frac{\gamma}{2\cdot \ell \cdot \eta}\big)^{2\ell+2}$)
 to obtain that 
 \[
 \Vert \Sigma^{-1/2} - \widetilde{\Sigma}^{-1/2} \Vert \leq \frac{\delta}{2 \big( \frac{\gamma}{2\cdot \ell \cdot \eta}\big)^{\ell+1}}. 
 \]
 Now, set $\delta = 2 \frac{\epsilon}{\ell \cdot \eta} \cdot \big( \frac{\gamma}{2\cdot \ell \cdot \eta}\big)^{\ell+1}$. Define $\alpha_{i,j} = \widetilde{\Sigma}^{-\frac12}(i,j)$, the second item now follows immediately. For the first item, observe that by Weyl's inequality (Lemma~\ref{lem:Weyl}), $\sigma_{\min}(\widetilde{\Sigma}) \ge  (1-\delta) \cdot \sigma_{\min}({\Sigma})$. Thus, $$\Vert \widetilde{\Sigma}^{-1} \Vert_F \le \bigg(\frac{2 \ell \eta}{\gamma}\bigg)^{\ell+1} \cdot \ell \cdot \eta.$$
Finally, since $\widetilde{\Sigma}^{-1/2}$ is also Hermitian, it is easy to see that 
\[
\Vert \widetilde{\Sigma}^{-1/2} \Vert_F  \le \sqrt{\ell} \cdot \sqrt{\Vert \widetilde{\Sigma} \Vert_F}.  
\] 
This puts an upper bound on $|\alpha_{i,j}|$ finishing the proof. 
 %Then, by Weyl's inequality (Lemma~\ref{lem:Weyl}), $\sigma_{\min}(\widetilde{\Sigma}) \ge  (1-\delta) \cdot \sigma_{\min}({\Sigma})$. {\color{red}We now recall a couple of standard matrix perturbation bounds. }
\end{proof}
%\begin{lemma}~\label{lem:Lipschitz-closeness}
%Let $f: \mathbb{R}^n \rightarrow \mathbb{R}$ which is a linear $k$-junta and $\mathsf{surf}(f) \le s$. 
%\end{lemma}
%\begin{lemma}~\label{lem:Lip-2}
%Let $g: \mathbb{R}^n \rightarrow [-1,1]$ and let $P_t g$ be $\epsilon$-close to a $W$-junta where $\mathsf{dim}(W)=k$. 
%\end{lemma}
\begin{proposition}~\label{prop:sing-1}
Let $v_1, \ldots, v_\ell$ be a $(\eta, \gamma)$-linearly independent vectors.  Let $V = [v_1 | \ldots | v_\ell]$. Then, the smallest singular value of $V$
is at least $(\frac{ \gamma}{2 \cdot \ell \cdot \eta})^{\ell+1}$. 
\end{proposition}
\begin{proof}
Let $\kappa>0$ whose precise value will be fixed later.
Now, note that if $\sigma_{\min}$ is the smallest singular value of $V$, then $\inf_{x : \Vert x \Vert_2=1} \Vert V \cdot x \Vert_2$. In order to lower bound this, observe that $V \cdot x = \sum_{1 \le i \le \ell} v_i \cdot x_i$. 
Now, let $j$ be the largest coordinate such that $|x_j| \ge \kappa^{j}$ (note that there has to be such a $j$ since $x$ is a unit vector). Define $w = \sum_{i \le j} v_i x_i$. Then, observe that its component in the direction orthogonal to the span of $\{v_1, \ldots, v_{j-1}\}$ is at least $\gamma \cdot \kappa^j$ in magnitude. On the other hand, $\Vert \sum_{i > j} v_i x_i \Vert_2 \le \kappa^{j+1} \cdot \ell \cdot \eta$. Now, as long as  $\kappa \le \frac{\gamma}{2 \cdot \ell \cdot \eta}$, we obtain that 
\[
\Vert \sum_{i} v_i x_i \Vert_2 \ge \Vert \sum_{i \le j} v_i x_i \Vert_2 - \Vert \sum_{i >  j} v_i x_i \Vert_2 \ge \gamma \cdot \kappa^j - \ell \cdot \eta \cdot \kappa^{j+1}  \ge  \frac{\gamma \cdot \kappa^j}{2}. 
\]
This finishes the proof.
\end{proof}

\begin{lemma}~\label{lem:test-one}
There is a routine \textsf{Test-closeness-one} such that given oracle access to $f: \mathbb{R}^n \rightarrow [-1,1]$, $(y_1, \ldots, y_\ell)$ which are $\gamma$-linearly independent for $P_t f$ and access to 
$g \in \mathsf{Cover}(t,\ell,\epsilon)$, has the following guarantee: 
\begin{enumerate}
\item For $\tau = \epsilon^2/(100 \cdot \ell^{3/2})$, it makes $T(\tau, t,\gamma) \cdot \log(1/\xi)$ queries to $f$ (where $T(\cdot, \cdot, \cdot)$ 
is the function in Lemma~~\ref{lem:apx-ortho}). 
\item There is an orthonormal basis $(w_1, \ldots, w_\ell)$ of $\mathsf{span}(Dh_{y_1}(y_1), \ldots, Dh_{y_\ell}(y_\ell))$ (which depends just on that) such that
with probability $1-\xi$, the algorithm outputs an $\epsilon/100$ accurate estimate to $\mathbf{E}[\Vert P_t f - g (w_1, \ldots ,w_\ell) \Vert_1]$. 
\end{enumerate}
\end{lemma}
\begin{proof}
First, we run the procedure in  Lemma~\ref{lem:apx-ortho}with error parameter $\tau$, noise rate $t$ and parameter $\gamma$. Note that with $T(\tau, t, \gamma)$ queries, we are able to obtain coefficients $\{\alpha_{i,j} \} $ such that 
\begin{equation}~\label{eq:bound-tau}
\Vert \sum_{j} \alpha_{i,j} Dh_{y_j}(y_j) -w_i \Vert_2 \le \tau. 
\end{equation}
Let $K = \sum_{i,j} |\alpha_{i,j}|$. Set the parameter $\eta= \frac{\epsilon^2}{K \cdot \ell}$. 
Let us now define a point $x \in \mathbb{R}^n$ to be \emph{good} if the following holds: 
\begin{enumerate}
\item For all $1 \le i \le \ell$, the function $f_{\partial, \eta, t, y_i}$ defined in Lemma~\ref{lem:compute-derivative-x}, 
$$
\big| f_{\partial, \eta, t, y_i} (x) - \langle D_{y_i} (P_tf)(y_i), x \rangle \big| \le \frac{\ell \cdot \eta}{\epsilon}. 
$$ 
\item For all $1 \le i \le \ell$, 
$$
\big| \sum_{j} \alpha_{i,j} \langle Dh_{y_j}(y_j),x \rangle - \langle w_i, x\rangle \big| \le \frac{\epsilon}{100 \ell}. 
$$ 
\end{enumerate} 
The crucial point is that for a randomly chosen $x \sim \gamma_n$, Lemma~\ref{lem:compute-derivative-x}  guarantees that the first item is satisfied with probability at least $1 - \frac{\epsilon^2}{\ell \cdot \eta^2}$. Likewise, from (\ref{eq:bound-tau}), for $x \sim \gamma_n$, we get that the second item is satisfied with probability $\epsilon/(100\ell)$. Thus, we get that a point $x \sim \gamma_n$ is \emph{good} with probability $1-\epsilon/\ell$. The algorithm \textsf{Test-closeness-one} is now defined as follows: 
\begin{enumerate}
\item Sample $s = 1/\epsilon^2 \cdot \log(1/\xi)$ points $x_1, \ldots, x_s$. 
\item For each of the points $x_i$, do the following: 
\item \hspace*{10pt} Compute $f_{\partial, \eta, t, y_j}(x_i)$ for $1 \le j \le \ell$ up to error $\frac{\epsilon}{K \cdot \ell}$. 
\item \hspace*{10pt} Compute $\tilde{\beta}_{i,x} = \sum_{j} \alpha_{i,j}f_{\partial, \eta, t, y_j}(x_i)$. 
\item  \hspace*{10pt} Compute $g(\tilde{\beta}_{1,x} ,\ldots, \tilde{\beta}_{\ell,x})$. 
\item Output $\frac{1}{s} \sum_{i=1}^s |P_tf(x_i) - g(\tilde{\beta}_{1,x} ,\ldots, \tilde{\beta}_{\ell,x})|$. 
\end{enumerate}

The analysis of this algorithm is as follows: 
\begin{eqnarray*}
&& \big|\mathbf{E}_{x \sim \gamma_n}\big[ |P_tf(x_i) - g(\tilde{\beta}_{1,x} ,\ldots, \tilde{\beta}_{\ell,x})| \big]-\mathbf{E}_{x \sim \gamma_n}\big[ |P_tf(x_i) - g(\langle w_1,x\rangle ,\ldots, \langle w_\ell,x\rangle)| \big] \big| \\ &\le& \mathbf{E}_{x \sim \gamma_n} \big[ |g(\tilde{\beta}_{1,x} ,\ldots, \tilde{\beta}_{\ell,x})- g(\langle w_1,x\rangle ,\ldots, \langle w_\ell,x\rangle)| \big]
\end{eqnarray*}
Now, note that because $g$ is bounded by $[-1,1]$, the term inside the expectation is bounded by $2$. Further, if a point $x$ is \emph{good}, for every $1 \le i \le \ell$, 
$$
\big|\widetilde{\beta}_{i,x} - \langle w_i, x \rangle \big| \le \frac{\epsilon}{50 \ell}. 
$$
Now, this immediately implies that
\[
\mathbf{E}_{x \sim \gamma_n} \big[ |g(\tilde{\beta}_{1,x} ,\ldots, \tilde{\beta}_{\ell,x})- g(\langle w_1,x\rangle ,\ldots, \langle w_\ell,x\rangle)| \big] \le \frac{\epsilon}{50} + \Pr[x \textrm{ is not good}] \le \frac{\epsilon}{2}. 
\]
Item 2 now follows immediately.

%Choose any point $x \in \mathbb{R}^n$. Then, observe %that  
%$$
%\big| \sum_{j} \alpha_{i,j} \langle Dh_{y_j}(y_j),x %\rangle - \langle w_i, x\rangle \big| \le \tau \cdot \Vert x \Vert_2. 
%$$ 
%Thus, as long as $\Vert x \Vert_2 \le \sqrt{\ell} \cdot \log(1/\epsilon)$, we have that 
%$$
%\big| \sum_{j} \alpha_{i,j} \langle Dh_{y_j}(y_j),x \rangle - \langle w_i, x\rangle \big| \le \frac{\epsilon}{100 \ell}. 
%$$
\end{proof}
